# Supplementary material for: Dynamically polarisable force-fields for surface simulations via multi-output classification Neural Networks
Source: arXiv:2103.16447 ancillary file (2021-03-30)
Supplement: Supplementary file 1 [file SI.pdf]

# Supporting Information for "Dynamically polarisable force-fields for surface simulations via multi-output classification Neural Networks"

Nicodemo Di Pasquale,[*,†] Joshua D. Elliott,[†] Panagiotis Hadjidoukas,[‡] and Paola Carbone[†]

†*Department of Chemical Engineering and Analytical Science, University of Manchester, Manchester M13 9AL, United Kingdom*

‡*IBM Research, Zürich, Switzerland*

E-mail: nicodemo.dipasquale@manchester.ac.uk

## S.1 QM/MD Polarized Graphene layer

We present a brief description of the simulation we used to derive the training points for the construction of the neural network, for more details we refer to our original work[1]. The system under investigation is a charged semi-infinite graphene electrode in contact with a 1M NaCl electrolyte solution. The electrode is composed by 336 carbon atoms and carries an excess charge of 4 $e$. The electrolyte solution has 2065 water molecules and 90 and 86 fully dissociated $Na^+$ and $Cl^-$ ions respectively. It should be noted that the excess of Na ions balances the charge of the electrode, preventing problems with the computation of long-ranged electrostatic interactions in the MD step. The dimensions of the simulation box are approximately $3 \times 3 \times 16$ nm$^3$, where in the system non-periodic direction (orthogonal to the electrode plane) there is an 8 nm slab of electrolyte plus a further 8 nm of vacuum separating

periodic images.

For classical molecular dynamics simulations we use the GROMACS[2] software suite version 2018.4.

The surface polarization evolves in response to the local electrostatic potential of the water molecules and ions in solution, but it represents a quantum mechanical property of the surface electrons. In order to capture the redistribution of the electron density we iteratively couple density functional tight binding simulations of the graphene surface to the classical molecular dynamics trajectory. In practice we convert the coordinates of the electrolyte atoms (Hydrogen , Oxygen, Sodium and Chloride) from a snapshot of the classical trajectory into a set of point charges; the magnitude of the charge is taken from the classical force-field. The point charges form the background electrostatic potential for DFTB simulation of the graphene surface. The DFTB simulation in turn gives rise to a distribution of the surface electron density in response to the position of the electrolyte. From the distribution of the electron density we estimate the atomic charges through mulliken populations of the atomic orbitals. These atomic charges define the charges used in the classical force field for the generation future configurations. For the aqueous graphene interfaces we find that a coupling time of 5 ps between quantum mechanical feedback is sufficient for keeping the error in the atomic charges below 0.015 e.

From these calculations we obtained 30000 different configuration saved every 1 ps to reduce the correlation among the different geometries.

## S.2 Neural Network with Tensorflow

The NN model was obtained using Tensorflow/Keras library v. 2.3.1. We started with a set composed by 30000 configurations. Each configuration includes the positions and charges of the ions and the charges on the graphene layer, as input and output features, respectively. Therefore, the number of input features of each configurations is 704, calculated as: (number

of $Cl^-$ + number of $Na^+$ ) times four, for the three spatial coordinates and the charge of each ion.

We randomly split the total set of configurations in a training set composed by 27000 configurations and the holdout/test set with the remaining ones. Moreover, we use 10-fold cross validation, by diving the training set into 10 subsets and repeating the model training 10 times, with a single subset as holdout/test set.

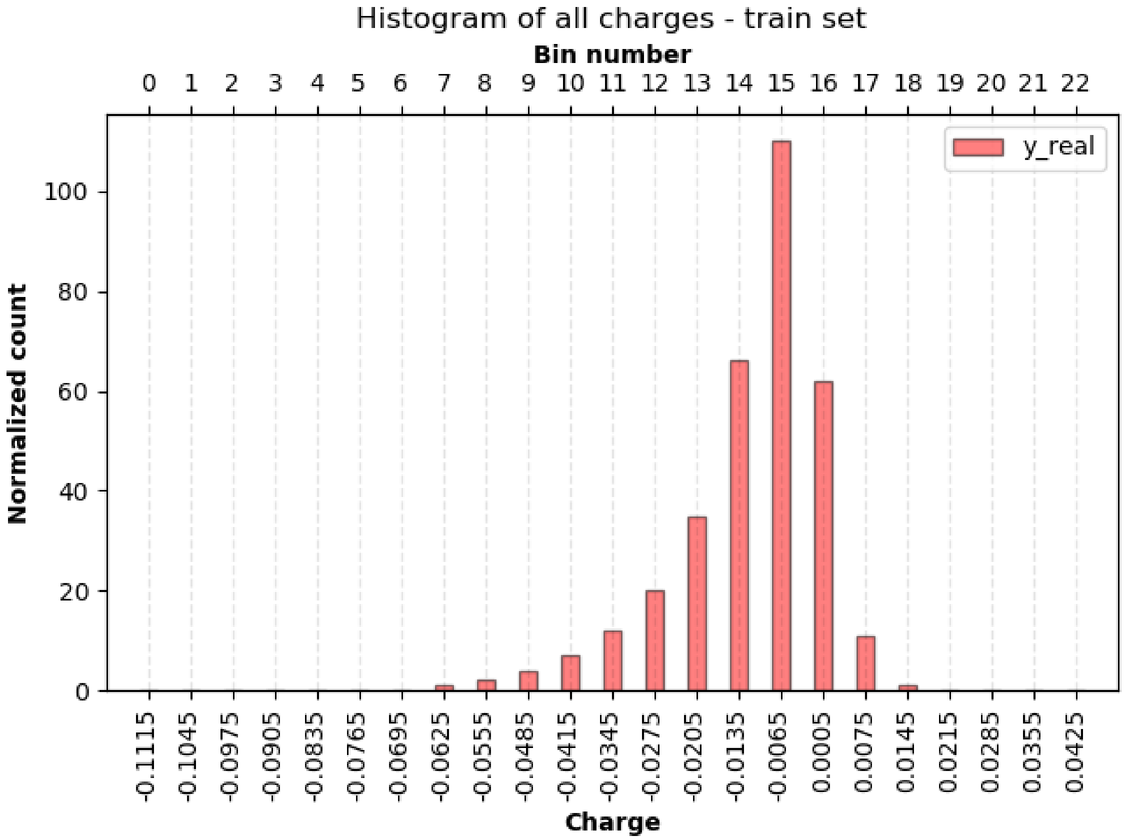


Figure S.1: Histogram of the distribution of charges on the carbon atoms of the electrode obtained from 27000 training geometries. The hystogram is normalized in the sense that the sum of all the bins gives the total number of carbons atoms considered on the electrode.

From the 27000 configurations in the training set, we built the histogram showing the relative frequency of the charges which is reported in fig. S.1. The spacing of the bins of this histogram was chosen to be $s_b = 0.007e$. The choice of the bin spacing has some important consequences for our work and we will describe it in more detail in the next section (see section S.2.1). The charge of the $k$-th carbon, $q_k$, was then assigned to $n_b^k$-th bin of the

histogram, according to:

$$n_b^k = \left\lceil \frac{q_k - q_{\text{min}}}{q_{\text{max}} - q_{\text{min}}} \right\rceil \tag{S.1}$$

where $q_{\text{max}}$ and $q_{\text{min}}$ are determined by the smallest and largest charges encountered in the 27000 points of the training set.

Multi-output/multi-target classification is not directly supported by NNs. Therefore, we built a multi-output regression NN and explicitly round the floating point predictions to integers, i.e. the discrete charge bin numbers. In turn, these bin numbers can be mapped to the actual charge values.

The NN is a typical multilayer perceptron (MLP) with four fully-connected dense hidden layers of 1024 neurons with *ReLU* activation. The custom loss function that combines the normal mean absolute error loss and the loss that penalizes the differences between the sum of real and predicted values is depicted in Listing 1.

The training is performed with the Adam() optimizer with initial learning rate $lr$=2e-4. Moreover, the training is automatically stopped with an early stopping mechanism if no improvement of the validation loss has been observed after 100 epochs.

```
def custom_loss(y_true, y_pred):
  # MAE loss
  err = K.mean(K.abs(y_true-y_pred), axis=-1)
  # Penalization of differences between sum(y_true) and sum(y_pred)
  fac = 1.0/336.0
  constraint = fac*K.abs(K.sum(y_pred, axis=-1)-K.sum(y_true, axis=-1))

  return(err+constraint)
```

Listing 1: Custom Loss Function defined in Eq. 3 of the main paper.

### S.2.1 Bin definition

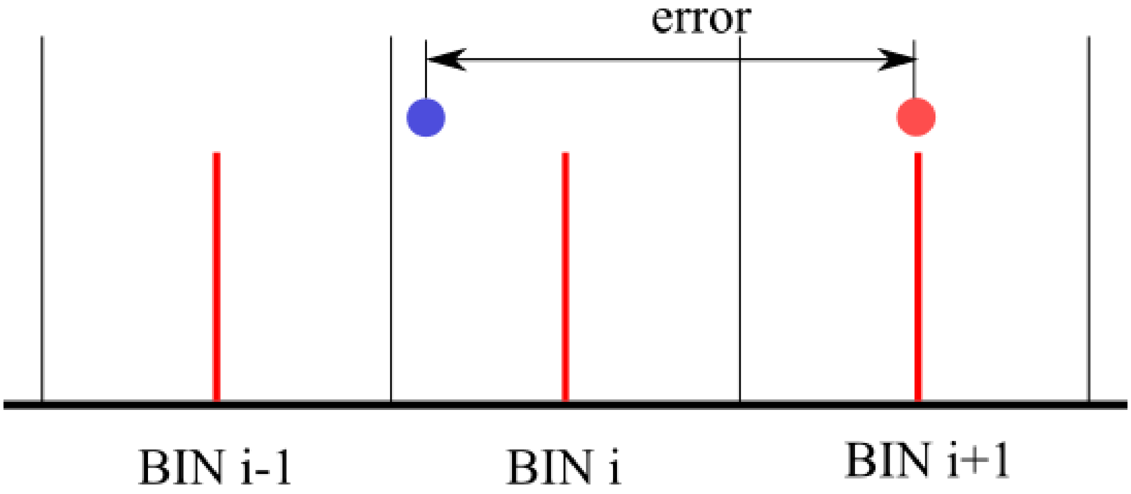


Figure S.2: Sketch of the assignment of the charges into the bins. Blue dot is the real charge, which is replaced with the value of the charge assigned to the bin $i$ (represented by the red line in bin $i$). Red dot is the predicted charge which is predicted in the wrong bin $i+1$. if the spacing between bins is greater than half of the threshold (see Sec. I of the main paper), then the prediction is not correct. Bu choosing a bin size smaller than half of the threshold, the prediction in the bin $i+1$ is still correct .

Once a given charge is assigned to one of the bins, it is replaced by the median value of that bin. In order to illustrate this point, in fig. S.2, we show one possible scenario for the prediction of the charges. The real charge is represented by the blue dot, and it can be anywhere in the region bounded by the upper and lower extrema of the bin. This latter fact puts a constraint on the maximum size of the bin, which has to be such that $b < \epsilon$.

If the predicted value, represented by the red dot in fig. S.2, is in the bin $i+1$, then the median value for the charge of the bin $i+1$ is assigned. If the size of the bin is $\epsilon$, the difference between the real charge (the blue dot) and the predicted charge (the red dot) is greater than $\epsilon$ and the prediction is wrong. If we use a spacing between the bins such that $b < e/2$ we can assume that the wrongly predicted label, with a difference of $\pm 1$ from the real one, is actually correct. In this work we consider $b = 0.007$.

# References


(1) Elliott, J. D.; Troisi, A.; Carbone, P. A QM/MD coupling method to model the ion-induced polarization of graphene. *J. Chem. Theory Comput.* **2020**, *16*, 5253–5263.

(2) Abraham, M. J.; Murtola, T.; Schulz, R.; Páll, S.; Smith, J. C.; Hess, B.; Lindahl, E. GROMACS: High performance molecular simulations through multi-level parallelism from laptops to supercomputers. *SoftwareX* **2015**, *1*, 19–25.
